# Supplementary material for: Neural View Synthesis and Matching for Semi-Supervised Few-Shot Learning of 3D Pose
Source: arXiv:2110.14213 source file (2021-10-27)
Supplement: Supplementary file 1 [file supplementary.tex]

% Code
% 7 manually selected images for each class
